# Supplementary material for: Merging Parameter Estimation and Classification Using LASSO
Source: arXiv:2405.03783 source file (2024-09-16)
Supplement: Supplementary file 1 [file Appendix.tex]

\section{Proof of Theorem 1}\label{sec:Appendix}

\begin{definition}

Define  \begin{equation}
    f^{(2)}(\theta_1,\theta_2)=\|\theta_2-\theta_1\|_2,
    \label{equ:k=2}
\end{equation}

and 

\begin{equation}
\begin{aligned}
    f^{(K)}(\theta_1,\cdots,\theta_K)&=f^{(K-1)}(\theta_1,\cdots,\theta_{K-1})\\
    &+\sum_{i=1}^{K-1}\|\theta_{K}-\theta_{i}\|_2, \quad \quad K\geq 3.
    \label{equ:intergroup}
\end{aligned}
\end{equation}

% and for short

% $g_K(\bar{\theta}^K):=f^{(K)}(\theta_1,\cdots,\theta_K)$, where $\bar{\theta}^K=(\theta_1,\cdots,\theta_K)$.

% $g_K(\theta_K):  \mathbb{R}^{n_{\theta}} \to \mathbb{R}$, $k\in \{1,\cdots,K\}$.

% Consider $g_k(\theta_k):=f^{(K)}(\theta_1,\cdots,\theta_K)$, $g_k(\theta_k):  \mathbb{R}^{n_{\theta}} \to \mathbb{R}$, $k\in \{1,\cdots,K\}$, which is defined as:

% \begin{equation}
% \begin{aligned}
%     f^{(K)}(\theta_1,\cdots,\theta_K)&=f^{(K-1)}(\theta_1,\cdots,\theta_{K-1})\\
%     &+\sum_{i=1}^{K-1}\|\theta_{K}-\theta_{i}\|_2, \quad \quad K\geq 3.
%     \label{equ:intergroup}
% \end{aligned}
% \end{equation}

% When $K=2$,

% \begin{equation}
%     f^{(2)}(\theta_1,\theta_2)=\|\theta_1-\theta_2\|_2.
%     \label{equ:k=2}
% \end{equation}

% When $K=1$, $f^{(1)}(\theta_1)$ doesn't exist.
    
\end{definition}

\begin{definition}

Let  $h_{ik}(\theta_1, \cdots, \theta_K)=\theta_i-\theta_k$, for $k<i, i \leq K$.
Define $z_{ik}$ as the sub-differential of $\| h_{ik} \|_2$ at a point where $\theta_i=\theta_k$.

% 0 for $n\in \{1,\cdots,\binom{K}{2}\}$, $z_n: \mathbb{R}^{n_{\theta}} \to \mathbb{R}$, $h_n: \mathbb{R}^{n_{\theta}\times n_{\theta}} \to \mathbb{R}^{n_{\theta}}$, $h_n=\theta_i-\theta_k$, and $i, k\in \{1,\cdots,K\}$. 
  
\end{definition}

Notice that $z_{ik}$ does not depend on the point where the sub-differential is taken.

Also notice that there are $\binom{K}{2}$ functions $h_{ik}$.

%$h_{ik}$ shows choose arbitrary 2 parameters $\theta_k$, and $k= 1,\cdots,K$. Thus, $n\in \{1,\cdots,\binom{K}{2}\}$. Take $G(\theta)=\|\theta_1-\theta_2\|_2+\|\theta_3-\theta_1\|_2$ as an example. Suppose $\theta_1=\theta_2=\theta_3$, we obtain $z_1$, $z_2$ are the sub-differential of $\|\theta_1-\theta_2\|_2$, and $\|\theta_3-\theta_1\|_2$ at 0, respectively. 

\begin{definition}
Define $p_K^k$ as the sub-differential of $f^{(K)}(\theta_1,\cdots,\theta_K)$ with respect to $\theta_k$ for $k\in \{1,\cdots,K\}$, $p_K^k: \mathbb{R}^{n_{\theta}\times K} \to \mathbb{R}$. 

\end{definition}

As illustration, take $f^{(3)}(\theta_1,\theta_2,\theta_3)=\|\theta_2-\theta_1\|_2+\|\theta_3-\theta_1\|_2 + \|\theta_3-\theta_2\|_2$. $p_3^1$ is the sub-differential of $f^{(3)}(\theta_1,\theta_2,\theta_3)$ with respect to $\theta_1$, and using that $f^{(3)}(\theta_1,\theta_2,\theta_3)$ is a composite function, we obtain $p_3^1=(-1)\cdot z_{21}+(-1)\cdot z_{31}=-z_{21}-z_{31}$. Similarly, we obtain $p_3^2=z_{21}-z_{32}$, and $p_3^3=z_{31}+z_{32}$.

\begin{lemma} [\cite{ohlsson2010segmentation}]
The sub-differential of $\| \cdot \|_{\rm{reg}}$ at 0 is the unit ball in the dual norm $\| \cdot \|_{\rm{reg*}}$, the regularization norm $\| \cdot \|_{\rm{reg}}$ could be any vector of norm . 
\end{lemma}

According to the lemma, it is easy to show that:

\begin{equation}
    z_{ik} \in \overline{B}(0,1,\|\cdot\|_*),
    \label{equ:1}
\end{equation}
where, $\overline{B}(0,1,\|\cdot\|_*)$ represents a sphere with 0 as the center and 1 as the radius.

\begin{definition}[\cite{boyd2004convex}]
Dual norm : Let $\| \cdot \|$  be a norm on $\mathbb{R}^n$. The associated dual norm, denoted $\| \cdot \|_*$, is defined as:

\begin{equation}
    \|z\|_*=\mathrm{sup}{\{z^Tx|\|x\|\leq 1\}}.
\end{equation}

\end{definition}

From the Cauchy-Schwarz inequality; for nonzero $z$, the value of $x$ that maximizes $z^Tx$ over $\|x\|\leq 1$ is $z/\|z\|_2$. Hence,

\begin{equation}
   \mathrm{sup}{\{z^Tx|\|x\|_2\leq 1\}}=\|z\|_2.
\end{equation}

Hence, we can conclude that the dual norm of the $\ell_2$-norm is itself, which we will use later in this proof.

%In this paper, we use $\ell_2$-norm, and it is easy to verify that the dual norm of a $\ell_2$-norm is itself ($\|\cdot\|_{2*}=\|\cdot\|_{2}$).

%The equation \eqref{equ:1} demonstrates that the sub-differential of $\theta_k$ is inside the sphere $\overline{B}$.

Focus on the model fit (the first term) and the clustering (the second term), the objective function is:

\begin{equation}
    \mathop{\min}_{\theta_k} \sum_{k=1}^K \|Y_k-\Phi_k \theta_{k}\|_2^2 +\frac{1}{2} \lambda_1\sum_{k,i=1}^{K,K}\|\theta_{k}-\theta_{i}\|_2.
     \label{equ:inter}
\end{equation}

The target of this work is to derive an upper bound $\lambda_{\mathrm{1max}}$ of the clustering term penalty coefficient $\lambda_1$. When $\lambda_1$ is larger than this bound, the parameter $\theta_k$ is constant. Assume $\lambda_{\mathrm{1max}}$ exists, then $\theta_1=\cdots=\theta_k=\cdots=\theta_K$.

Substituting \eqref{equ:intergroup} and \eqref{equ:k=2} into \eqref{equ:inter} yields:

\begin{equation}
    \mathop{\min}_{\theta_k} \sum_{k=1}^K \|Y_k-\Phi_k \theta_{k}\|_2^2 + \lambda_1 f^{(K)}(\theta_1,\cdots,\theta_K), K\geq 2.
     \label{equ:inter_new}
\end{equation}

Take K=3 as an example,

\begin{equation}
\begin{aligned}
\footnotesize
    f^{(3)}(\theta_1,\theta_2,\theta_3)
    &=f^{(2)}(\theta_1,\theta_2)+\sum_{i=1}^{2}\|\theta_{3}-\theta_{i}\|_2,\\
    &=\|\theta_2-\theta_1\|_2+\|\theta_3-\theta_1\|_2+\|\theta_3-\theta_2\|_2.
\end{aligned}
\end{equation}

Next, we derive $p_3^k$, which is the sub-differential of $f^{(3)}(\theta_1,\theta_2,\theta_3)$ evaluated at $\theta_k$ for $k\in \{1,2,3\}$.

\begin{equation}
\begin{aligned}
    p_3^1&=-z_{21}-z_{31},\\
    p_3^2&=z_{21}-z_{32},\\
    p_3^3&=z_{31}+z_{32}.\\
\end{aligned}
\end{equation}
%where $p_3^1$, $p_3^2$, and $p_3^3$ are the sub-differential of $f^{(3)}(\theta_1,\theta_2,\theta_3)$ evaluated at $\theta_1$, $\theta_2$, and $\theta_3$, respectively. $z_1$, $z_2$ and $z_3$ are the sub-differential at 0 for $\|\theta_1-\theta_2\|_2$,  $\|\theta_3-\theta_1\|_2$, and  $\|\theta_3-\theta_2\|_2$, respectively. 

Similarly, we can derive the general equations as shown in \eqref{equ:gen}. There are $K-1$ items for each $P_K^k$ when there exist $K$ parameters $\theta_k$.

\begin{equation}
\begin{aligned}
    f^{(K)}(\theta_1,\cdots,\theta_K)&=f^{(n-1)}(\theta_1,\cdots,\theta_{n-1})\\
    &+\sum_{i=1}^{K-1}\|\theta_{K}-\theta_{i}\|_2, \quad \quad K\geq 3.
    \label{equ:gen}    
\end{aligned}
\end{equation}

\begin{equation}
\begin{aligned}
    p_K^1&=-z_{21}-z_{31}-z_{41}-\cdots-z_{K1},\\
    p_K^2&=z_{21}-z_{32}-z_{42}-\cdots-z_{K2},\\
    p_K^3&=z_{31}+z_{32}-z_{43}-\cdots-z_{K3},\\
    & \vdots\\
    p_K^K&=z_{K1}+z_{K2}+z_{K3}+\cdots+z_{K(K-1)}.
    \label{equ:p}
\end{aligned}
\end{equation}

For working condition $k$, take the sub-differential of \eqref{equ:inter_new} with respect to $\theta_k$, and we get the necessary and sufficient conditions optimality

\begin{equation}
    2 \Phi_k[Y_k-\Phi_k^{\rm{T}} \cdot \theta_{k}]+ \lambda_1 \cdot p_K^k =0.
    \label{equ:opt}
\end{equation}

Combining \eqref{equ:opt} with \eqref{equ:p} yields for $k=K$

\begin{equation}
\begin{aligned}
        &2 \Phi_K[Y_K-\Phi_K^{\rm{T}} \cdot \theta_{K}]
        +\\
        &\lambda_1 \cdot ( z_{K1}+z_{K2}+z_{K3}+\cdots+z_{K(K-1)}) =0,
    \label{equ:total}
\end{aligned}
\end{equation}
where, $\| z_{ik} \|_{2*} \leq 1$, and $\theta_K$ is the optimal parameter. If there exists solution to \eqref{equ:total}

% . It doesn't matter which $k$ we choose, because in the following proof, we just use the length of $p_K^k$. Here, the number of the terms is $K-1$ for every $p_K^k$.

\begin{equation}
    2 \Phi_K[Y_K-\Phi_K^{\rm{T}} \cdot \theta_{K}]=-\lambda_1 \cdot ( z_{K1}+z_{K2}+z_{K3}+\cdots+z_{K(K-1)}).
    \label{equ:add3}
\end{equation}

Taking the norm of $\ell_2$-norm on both sides gives

\begin{equation}
\begin{aligned}
    &2\| \Phi_K[Y_K-\Phi_K^{\rm{T}} \cdot \theta_{K}]\|_{2}\\
    =&  \|\lambda_1 \cdot (z_{K1}+z_{K2}+z_{K3}+\cdots+z_{K(K-1)})\|_{2}.   
\end{aligned}
\end{equation}

Simplifying it, we have

\begin{equation}
\begin{aligned}
   &\|2 \Phi_K[Y_K-\Phi_K^{\rm{T}} \cdot \theta_{K}]/{\lambda_1}\|_{2}\\
   =& \|z_{K1}+z_{K2}+z_{K3}+\cdots+z_{K(K-1)}\|_{2}.    
   \label{equ:sim}
\end{aligned}
\end{equation}

% As the dual norm of a $\ell_2$-norm is itself, we derive:

% \begin{equation}
% \begin{aligned}
% &\left|\left|\frac{ 2 \Phi_K[Y_K-\Phi_K^{\rm{T}} \cdot \theta_{K}]}{\lambda_1}\right|\right|_{2}\\
% =&\left|\left|z_{\frac{K(K-1)+2}{2}}+\cdots+z_{\frac{K(K+1)}{2}}\right|\right|_{2}.
%     \label{minko}
% \end{aligned}
% \end{equation}

According to Minkowski's inequality,

\begin{equation}
    \begin{aligned}
         &\|z_{K1}+z_{K2}+z_{K3}+\cdots+z_{K(K-1)}\|_{2} \\ \leq & \|z_{K1}\|_{2}+\|z_{K2}\|_{2}+\|z_{K3}\|_{2}+\cdots +\|z_{K(K-1))}\|_{2}. 
    \end{aligned}
\end{equation}

 According to Lemma I.1., $\|z_{ik}\|_{2*} \leq 1$, and $\|\cdot\|_{2*}=\|\cdot\|_{2}$, thus $\|\cdot\|_{2}\leq 1$. Notice that there are $K-1$ items for each $P_K^k$ when there exist $K$ working conditions. Hence,

\begin{equation}
    \|z_{K1}\|_{2}+\|z_{K2}\|_{2}+\|z_{K3}\|_{2}+\cdots +\|z_{K(K-1))}\|_{2} \leq K-1.
    \label{equ:min}
\end{equation}

The derivations from \eqref{equ:sim} to \eqref{equ:min} give

\begin{equation}
    \|2 \Phi_K[Y_K-\Phi_K^{\rm{T}} \cdot \theta_{K}]/{\lambda_1}\|_{2} \leq K-1,
\end{equation}
which can be written

\begin{equation}
    \lambda_1 \geq \frac{2}{K-1} \| \Phi_K[Y_K-\Phi_K^{\rm{T}} \cdot \theta_K]\|_{2}.
\end{equation}

Similarly, using that the number of terms in $p_K^k$ is $K-1$, for $k\in \{1,\cdots,K\}$, we can derive:

\begin{equation}
    \lambda_{1} \geq \frac{2}{K-1} \| \Phi_k[Y_k-\Phi_k^{\rm{T}} \cdot \theta_k]\|_{2}.
    \label{eq:23}
\end{equation}

Recall that we are working on the assumptions that $\theta_1=\cdots=\theta_k=\cdots=\theta_K$. For this case, the solution is given by

\begin{equation}
    \theta_k=\theta_{\star}=\mathop{\rm{arg}\min}_{\theta} \sum_{k=1}^{K} \|Y_k-\Phi_k\theta\|_2^2, k=1,\cdots,K.
\end{equation}

Thus, the smallest $\lambda_1$ for which \eqref{eq:23} can hold is given by

\begin{equation}
\lambda_{1\rm{max}}=\max_{k\in \{1,\cdots,K\}}\left\{\frac{2} {K-1} \| \Phi_k[Y_k-\Phi_k^{\rm{T}} \cdot \theta_*]\|_{2} \right\},
\label{equ:max}
\end{equation}

which was to be proven.
